# Supplementary material for: A Weighted Exact Test for Mutually Exclusive Mutations in Cancer
Source: arXiv:1607.02447 source file (2016-07-08)
Supplement: Supplementary file 1 [file supplement.pdf]

# Supplement for A Weighted Exact Test for Mutually Exclusive Mutations in Cancer

Mark D.M. Leiserson, Matthew A. Reyna, Benjamin J. Raphael

Department of Computer Science and Center for Computational Molecular Biology, Brown University, Providence, 02912, USA

## S1 Introduction

In Section S2 of the supplement, we provide a partial derivation of the saddlepoint approximation for the WR-exclusivity $p$-value. In Section S3 of the supplement, we include additional figures and tables from the experiments in the manuscript, including

- the distributions of sample mutation frequencies for different cancer types,
- a comparison of the R-exclusivity test and the WR-exclusivity test with a weights given by the R-exclusivity test sample space $\Omega_{\mathrm{R}}$, and
- the top triples found by the R-exclusivity test and the WR-exclusivity test on thyroid cancer (THCA) with weights given by the RC-exclusivity test sample space $\Omega_{\mathrm{RC}}$.

## S2 Derivation of the saddlepoint approximation

In this section, we derive a saddlepoint approximation for the WR-exclusivity $p$-value for a set $M$ of $k$ events. Our approach applies to arbitrary sets $M$ of arbitrary size $k \geq 2$, but this derivation considers $k = 3$ for the ease of presentation.

Our approach is inspired by [3], who derive a saddlepoint approximation for a weighted enrichment test for differentially expressed genes in Gene Ontology categories, and it follows the approach of [1] in greater detail.

As described in the text of the manuscript, for our model, we assume that $\{X_{ij}\}_{j=1}^{n}$ is a set of mutually independent Bernoulli trials for each gene $g_i$ with success probabilities $W = [w_{ij}]$, i.e.,

$$\Pr(X_{ij} = \ell) = \begin{cases} w_{ij}, & \text{if } \ell = 1, \\ 1 - w_{ij}, & \text{if } \ell = 0, \end{cases} \tag{1}$$

where $w_{ij}$ is the probability that gene $g_i$ is mutated in sample $s_j$. Let $T_{M,j}$ be a random variable with $T_{M,j} = 1$ if $s_j$ has a mutually exclusive mutation in a gene set $M$ and $T_{M,j} = 0$ otherwise. Therefore, $Y_i = \sum_{j=1}^{n} X_{ij}$ is a Poisson binomial distributed variable for the number of mutations in $g_i$ and $T_M = \sum_{j=1}^{n} T_{M,j}$ is a test statistic for mutual exclusivity indicating the number of mutually exclusive mutations in $M$. We want to find the tail probability (commonly referred to as the $p$-value) of observing at least $t_M$ mutually exclusive mutations in $M$ given that $g_i$ is mutated in $r_i$ samples. The WR-exclusivity $p$-value $\Phi_{\text{WR}}(M)$ is the probability of observing at least $t_M$ mutations in a gene set $M$ under this model with

$$\Phi_{\text{WR}}(M) = \Pr(T_M \geq t_M \mid Y_M = \mathbf{r}_M) \tag{2}$$

where $Y_M = [Y_i]_{i \in M}$ and $\mathbf{r}_M = [r_i]_{i \in M}$.

The saddlepoint approximation is given by

$$\Pr(T_M \geq t_M \mid Y_M = \mathbf{r}_M) \approx 1 - \Phi(\tilde{w}) - \phi(\tilde{w}) \left( \frac{1}{\tilde{w}} - \frac{1}{\tilde{u}} \right), \tag{3}$$

where $\Phi$ and $\phi$ are, in this setting, the cumulative distribution and density functions, respectively, of the standard normal distribution, and $\tilde{w}$ and $\tilde{u}$ are defined as follows.

Without loss of generality, let $M = \{1, \dots, k\}$. First, for $\lambda \in \mathbb{R}^{k+1}$, let $\mathcal{M}_{Y_M,T_M}(\lambda) = E[e^{\sum_{i \in M} \lambda_i Y_i + \lambda_{k+1} T_M}]$ be the joint moment generating function of $\{Y_i\}_{i \in M}$ and $T_M$, and let $\mathcal{K}_{Y_M,T_M}(\lambda) = \log \mathcal{M}_{Y_M,T_M}(\lambda)$ be the corresponding joint cumulant generating function.

By the mutual independence of $\{Y_i\}_{i\in M}$, we have

$$\begin{aligned}
&K_{Y_M,T_M}(\lambda)\\
&\quad= \log E[e^{\lambda_1 Y_1+\lambda_2 Y_2+\lambda_3 Y_3+\lambda_4 T_M}]\\
&\quad= \log E[e^{\lambda_1 \sum_j X_{1,j}+\lambda_2 \sum_j X_{2,j}+\lambda_3 \sum_j X_{3,j}+\lambda_4 \sum_j T_{M,j}}]\\
&\quad= \log E[e^{\sum_j \lambda_1 X_{1,j}+\lambda_2 X_{2,j}+\lambda_3 X_{3,j}+\lambda_4 T_{M,j}}]\\
&\quad= \log \prod_{j=1}^{n} E[e^{\lambda_1 X_{1,j}+\lambda_2 X_{2,j}+\lambda_3 X_{3,j}+\lambda_4 T_{M,j}}]\\
&\quad= \sum_{j=1}^{n} \log E[e^{\lambda_1 X_{1,j}+\lambda_2 X_{2,j}+\lambda_3 X_{3,j}+\lambda_4 T_{M,j}}].
\end{aligned} \tag{4}$$

Note that $T_{M,j}$ can be written in terms of $\{X_{ij}\}_{i\in M}$. In this case, we have

$$\begin{aligned}
T_{M,j} = {} & X_{1j}(1-X_{2j})(1-X_{3j})\\
& + (1-X_{1j})X_{2j}(1-X_{3j}) + (1-X_{1j})(1-X_{2j})X_{3j}.
\end{aligned} \tag{5}$$

Since $\{X_{ij}\}$ are mutually independent and since the expected value of a Bernoulli random variable is equal to its success probability, we have

$$K_{Y_M,T_M}(\lambda) = \sum_{j=1}^{n} \log L^{(j)}_{Y_M,T_M}(\lambda), \tag{6}$$

where

$$\begin{aligned}
&L^{(j)}_{Y_M,T_M}(\lambda)\\
&\quad= E[e^{\lambda_1 X_{1,j}+\lambda_2 X_{2,j}+\lambda_3 X_{3,j}+\lambda_4 T_{M,j}}]\\
&\quad= (1-w_{1,j})(1-w_{2,j})(1-w_{3,j}) + e^{\lambda_1+\lambda_4} w_{1,j}(1-w_{2,j})(1-w_{3,j})\\
&\qquad + e^{\lambda_2+\lambda_4}(1-w_{1,j})w_{2,j}(1-w_{3,j}) + e^{\lambda_3+\lambda_4}(1-w_{1,j})(1-w_{2,j})w_{3,j}\\
&\qquad + e^{\lambda_1+\lambda_2} w_{1,j}w_{2,j}(1-w_{3,j}) + e^{\lambda_1+\lambda_3} w_{1,j}(1-w_{2,j})w_{3,j}\\
&\qquad + e^{\lambda_2+\lambda_3}(1-w_{1,j})w_{2,j}w_{3,j} + e^{\lambda_1+\lambda_2+\lambda_3} w_{1,j}w_{2,j}w_{3,j}.
\end{aligned} \tag{7}$$

Each of the above terms corresponds to one of the $2^k$ binary assignments for $\{X_{ij}\}_{i\in M}$, e.g., the term $(1-w_{1,j})(1-w_{2,j})(1-w_{3,j})$ corresponds to assignments $X_{1j} = X_{2j} = X_{3j} = 0$. For the simplicity of notation, let $L^{(j)}(\lambda) = L^{(j)}_{Y_M,T_M}(\lambda)$ for the rest of the derivation.

Similarly, let $\mathcal{M}_{Y_i}(\lambda) = E[e^{\lambda_i Y_i}]$ be the moment generating function of $Y_i$, and let $\mathcal{K}_{Y_i}(\lambda) = \log \mathcal{M}_{Y_i}(\lambda)$ be the corresponding cumulant generating function. The derivations for these quantities are similar.

Next, let $\mathcal{K}'_{Y_M,T_M}(\lambda)$ be the gradient vector of $\mathcal{K}_{Y_M,T_M}(\lambda)$. For example, we see that

$$\frac{\partial}{\partial \lambda_1} K_{Y_M,T_M}(\lambda) = \sum_{j=1}^{n} \frac{L^{(j)}_{\lambda_1}(\lambda)}{L^{(j)}(\lambda)}, \tag{8}$$

where

$$\begin{aligned} L^{(j)}_{\lambda_1} &= \frac{\partial}{\partial \lambda_1} L^{(j)}_{Y_M,T_M}(\lambda) \\ &= e^{\lambda_1+\lambda_4} w_{1,j}(1-w_{2,j})(1-w_{3,j}) + e^{\lambda_1+\lambda_2} w_{1,j} w_{2,j}(1-w_{3,j}) \\ &\quad + e^{\lambda_1+\lambda_3} w_{1,j}(1-w_{2,j}) w_{3,j} + e^{\lambda_1+\lambda_2+\lambda_3} w_{1,j} w_{2,j} w_{3,j}. \end{aligned} \tag{9}$$

The derivations for the remaining entries of $\mathcal{K}'_{Y_M,T_M}(\lambda)$ are similar.

Furthermore, let $\mathcal{K}''_{Y_M,T_M}(\lambda)$ be the Hessian matrix of $\mathcal{K}_{Y_M,T_M}(\lambda)$. For example, we see that

$$\frac{\partial^2}{\partial \lambda_1 \partial \lambda_2} K_{Y_M,T_M}(\lambda) = \sum_{j=1}^{n} \frac{L^{(j)}_{\lambda_1\lambda_2}}{L^{(j)}} - \frac{L^{(j)}_{\lambda_1} L^{(j)}_{\lambda_2}}{\left(L^{(j)}\right)^2}, \tag{10}$$

where $L^{(j)}_{\lambda_1}$ and $L^{(j)}_{\lambda_2}$ were already derived for the derivation of $\mathcal{K}'_{Y_M,T_M}$ and

$$\begin{aligned} L^{(j)}_{\lambda_1\lambda_2} &= \frac{\partial^2}{\partial \lambda_1 \partial \lambda_2} L^{(j)}_{Y}(\lambda) \\ &= e^{\lambda_1+\lambda_2} w_{1,j} w_{2,j}(1-w_{3,j}) + e^{\lambda_1+\lambda_2+\lambda_3} w_{1,j} w_{2,j} w_{3,j}. \end{aligned} \tag{11}$$

The derivations for the remaining entries of $\mathcal{K}''_{Y_M,T_M}(\lambda)$ are similar.

Finally, define $\tilde{w}$ by

$$\tilde{w} = \sqrt{2}\,\mathrm{sgn}\left(\tilde{y}_{k+1}\right) \sqrt{\sum_{i \in M} \mathcal{K}_{Y_i}(\hat{x}_i) - \mathcal{K}_{Y_M,T_M}(\tilde{y}) - \tilde{y}^T \left(\hat{x} - \tilde{x}\right)} \tag{12}$$

and $\tilde{u}$ by

$$\tilde{u} = 2 \sinh\left(\frac{\tilde{y}_{k+1}}{2}\right) \sqrt{\frac{\left|\mathcal{K}''_{Y_M,T_M}(\tilde{y})\right|}{\prod_{i \in M} \mathcal{K}''_{Y_i}(\hat{x}_i)}}, \tag{13}$$

where $\tilde{x} = \left(r_1, \ldots, r_k, t_M - \frac{1}{2}\right)$ and $\tilde{y} = (\tilde{y}_1, \ldots, \tilde{y}_{k+1})$ with $\tilde{y}$ the unique solution for $\mathcal{K}'_{Y_M,T_M}(\tilde{y}) = \tilde{x}$ and (3) undefined if $\tilde{y}_{k+1} = 0$, and $\hat{x} = (\hat{x}_1, \ldots, \hat{x}_k, 0)$ with $\hat{x}_i$ the unique solution for $\mathcal{K}'_{Y_i}(\hat{x}_i) = r_i$.

Note that, in general, $\mathcal{K}'_{Y_M,T_M}(\tilde{y}) = \tilde{x}$ is a system of $k+1$ nonlinear equations, and $\mathcal{K}'_{Y_i}(\hat{x}_i)$ is a sequence of $k$ nonlinear equations. A root finder, e.g., the MINPACK routine HYBRJ [4], can solve these systems of equations when given expressions for the gradient vector $\mathcal{K}'_{Y_M,T_M}(\lambda)$ and the Hessian matrix $\mathcal{K}''_{Y_M,T_M}(\lambda)$; the MINPACK routine HYBRD approximates $\mathcal{K}''_{Y_M,T_M}(\lambda)$. Various wrappers for HYBRJ and HYBRD exist in various languages, including SciPy's Python wrapper [2], which we used in our code.

## S3 Supplemental figures and tables

Figure S1 compares the number of mutated genes per sample in thyroid cancers (THCA), colorectal cancers (COADREAD), and endometrial carcinomas (UCEC), demonstrating high mutation rates in several COADREAD and UCEC samples and high mutational variability in COADREAD and UCEC data.

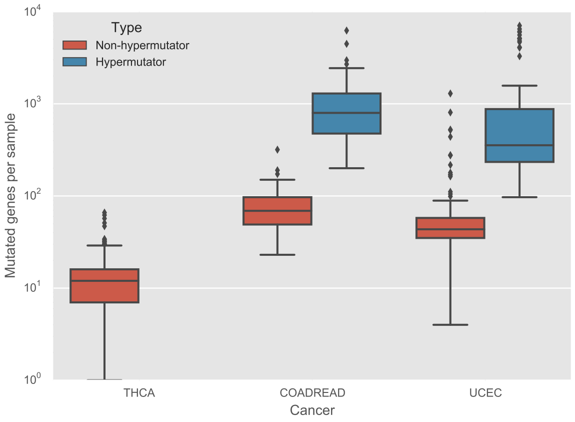


Figure S1: Boxplot of the number of mutated genes per sample in the THCA, COADREAD, and UCEC datasets. The COADREAD and UCEC samples are further broken down into hypermutators (blue) and non-hypermutators (red).

Figure S2 shows a comparison of the $p$-values and runtimes given by the recusive formula and the saddlepoint approximation methods. On these datasets, the saddlepoint approximation is an extremely accurate approximation of the tail enumeration procedure ($\rho^2 = 0.995$). Additionally, while the median runtimes of the two algorithms are similar, the tail enumeration

procedure is much slower for sets with co-occurring mutations while the saddlepoint approximation is largely unaffected. We expect the discrepancy between runtimes to grow for gene sets of larger sizes. Also, the saddlepoint approximation can be optimized when approximating the R-exclusivity test because each row of the corresponding weight matrix has identical entries, but we did not do so here.

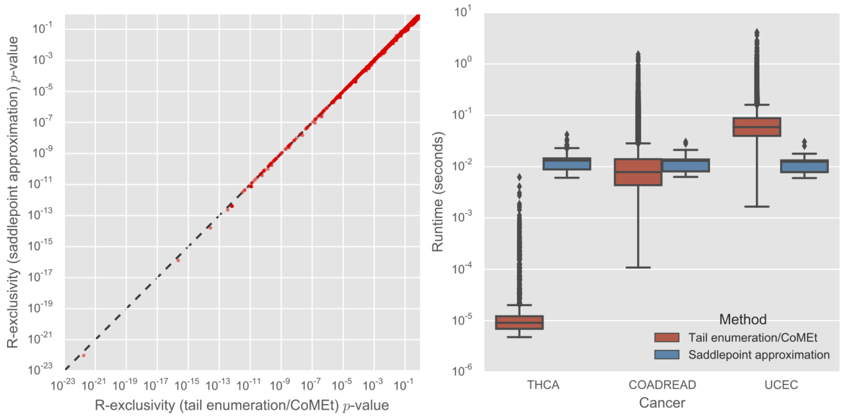


Figure S2: Comparison of the tail enumeration and saddlepoint approximation algorithms for computing the R-exclusivity $p$-value $\Phi_{\mathrm{R}}(M)$ on triples in THCA, COADREAD, and UCEC. (left) Scatter plot comparing the $p$-values given by the tail enumeration algorithm ($x$-axis) versus the saddlepoint approximation ($y$-axis). (right) Distribution of the runtime (in seconds) required to compute each method on a single triple.

Table S1 shows the five most significant triples identified by the R-exclusivity and WR-exclusivity tests on thyroid cancer (THCA).

| $\Phi_{\mathbf{R}}$ **rank** | $\Phi_{\mathbf{WR}}$ **rank** | **Triple** $M$ | $\Phi_{\mathbf{R}}(M)$ | $\Phi_{\mathbf{WR}}(M)$ |
|---|---|---|---|---|
| 1 | 1 | BRAF, HRAS, NRAS | $1.79 \cdot 10^{-22}$ | $1.79 \cdot 10^{-27}$ |
| 2 | 2 | BRAF, EIF1AX, NRAS | $2.27 \cdot 10^{-16}$ | $2.73 \cdot 10^{-20}$ |
| 3 | 3 | **BDP1**, BRAF, NRAS | $2.70 \cdot 10^{-14}$ | $6.01 \cdot 10^{-18}$ |
| 4 | 4 | BRAF, NRAS, TG | $3.51 \cdot 10^{-13}$ | $5.62 \cdot 10^{-17}$ |
| 5 | 5 | BRAF, **MUC5B**, NRAS | $6.58 \cdot 10^{-13}$ | $1.90 \cdot 10^{-16}$ |

Table S1: Five most significant triples identified by the R-exclusivity and WR-exclusivity tests on the THCA dataset. Genes in bold are among the 600 longest genes (at least 9,560 amino acids). Seven triples tie for the fifth smallest R-exclusivity $p$-value, so we indicate the triple with the smallest WR-exclusivity $p$-value in the table.

# References


[1] Ronald W Butler. *Saddlepoint approximations with applications*, volume 22. Cambridge University Press, 2007.

[2] Eric Jones, Travis Oliphant, Pearu Peterson, et al. SciPy: Open source scientific tools for Python, 2001–.

[3] David Manescu and Uri Keich. A Symmetric Length-Aware Enrichment Test. *RECOMB*, pages 224–242, 2015.

[4] Jorge J Moré, Burton S Garbow, and Kenneth E Hillstrom. User guide for minpack-1. Technical report, 1980.
